# Supplementary material for: Event-based Dynamic Graph Representation Learning for Patent Application Trend Prediction
Source: arXiv:2308.09780 source file (2023-09-05)
Supplement: Supplementary file 1 [file Appendix.tex]

\appendix
\label{section-appendix}
In the appendix, details of the experiments are introduced.
